# Supplementary material for: FairRec: Fairness-aware News Recommendation with Decomposed Adversarial Learning
Source: arXiv:2006.16742 source file (2021-04-15)
Supplement: Supplementary file 1 [file supplement.tex]

\section*{Supplementary Materials}

\subsection*{Hyperparameter Settings}
The settings of hyperparameters used in our approach are summarized in Table~\ref{hyper}.

\begin{table}[h]
\centering
\caption{Detailed hyperparameter settings.}\label{hyper}
%\resizebox{1.0\linewidth}{!}{
\begin{tabular}{|l|c|}
\hline
\multicolumn{1}{|c|}{\textbf{Hyperparameters}}& \textbf{Value} \\ \hline
word embedding dimension                     & 300            \\ 
\# heads in self-attention                 & 16             \\
output dim of each head               & 16            \\
negative sampling ratio $T$  & 4 \\ 
dropout                                      & 0.2            \\
$\lambda_G$                                  & 0.5            \\
$\lambda_D$                                  & 0.5            \\
$\lambda_A$                                  & 0.5            \\
optimizer                                    & Adam           \\
learning rate                                & 1e-3           \\
batch size                                   & 30    \\     \hline
\end{tabular}
%}

\end{table}

\subsection*{Results on Real Impression Logs}
The fairness performance of different methods on the real test impression logs is shown in Table~\ref{table.result3}. 
We can see that the randomly ranked results are also gender-discriminative (the performance is higher than majority and random prediction).
It shows that the impression logs are influenced by the system gender biases brought by news recall and ranking, which are not suitable for evaluating the fairness performance.

\begin{figure}[!t]
    \centering
    \subfigure[Adversarial learning only.]{\label{analysis1}
    \includegraphics[width=0.98\linewidth]{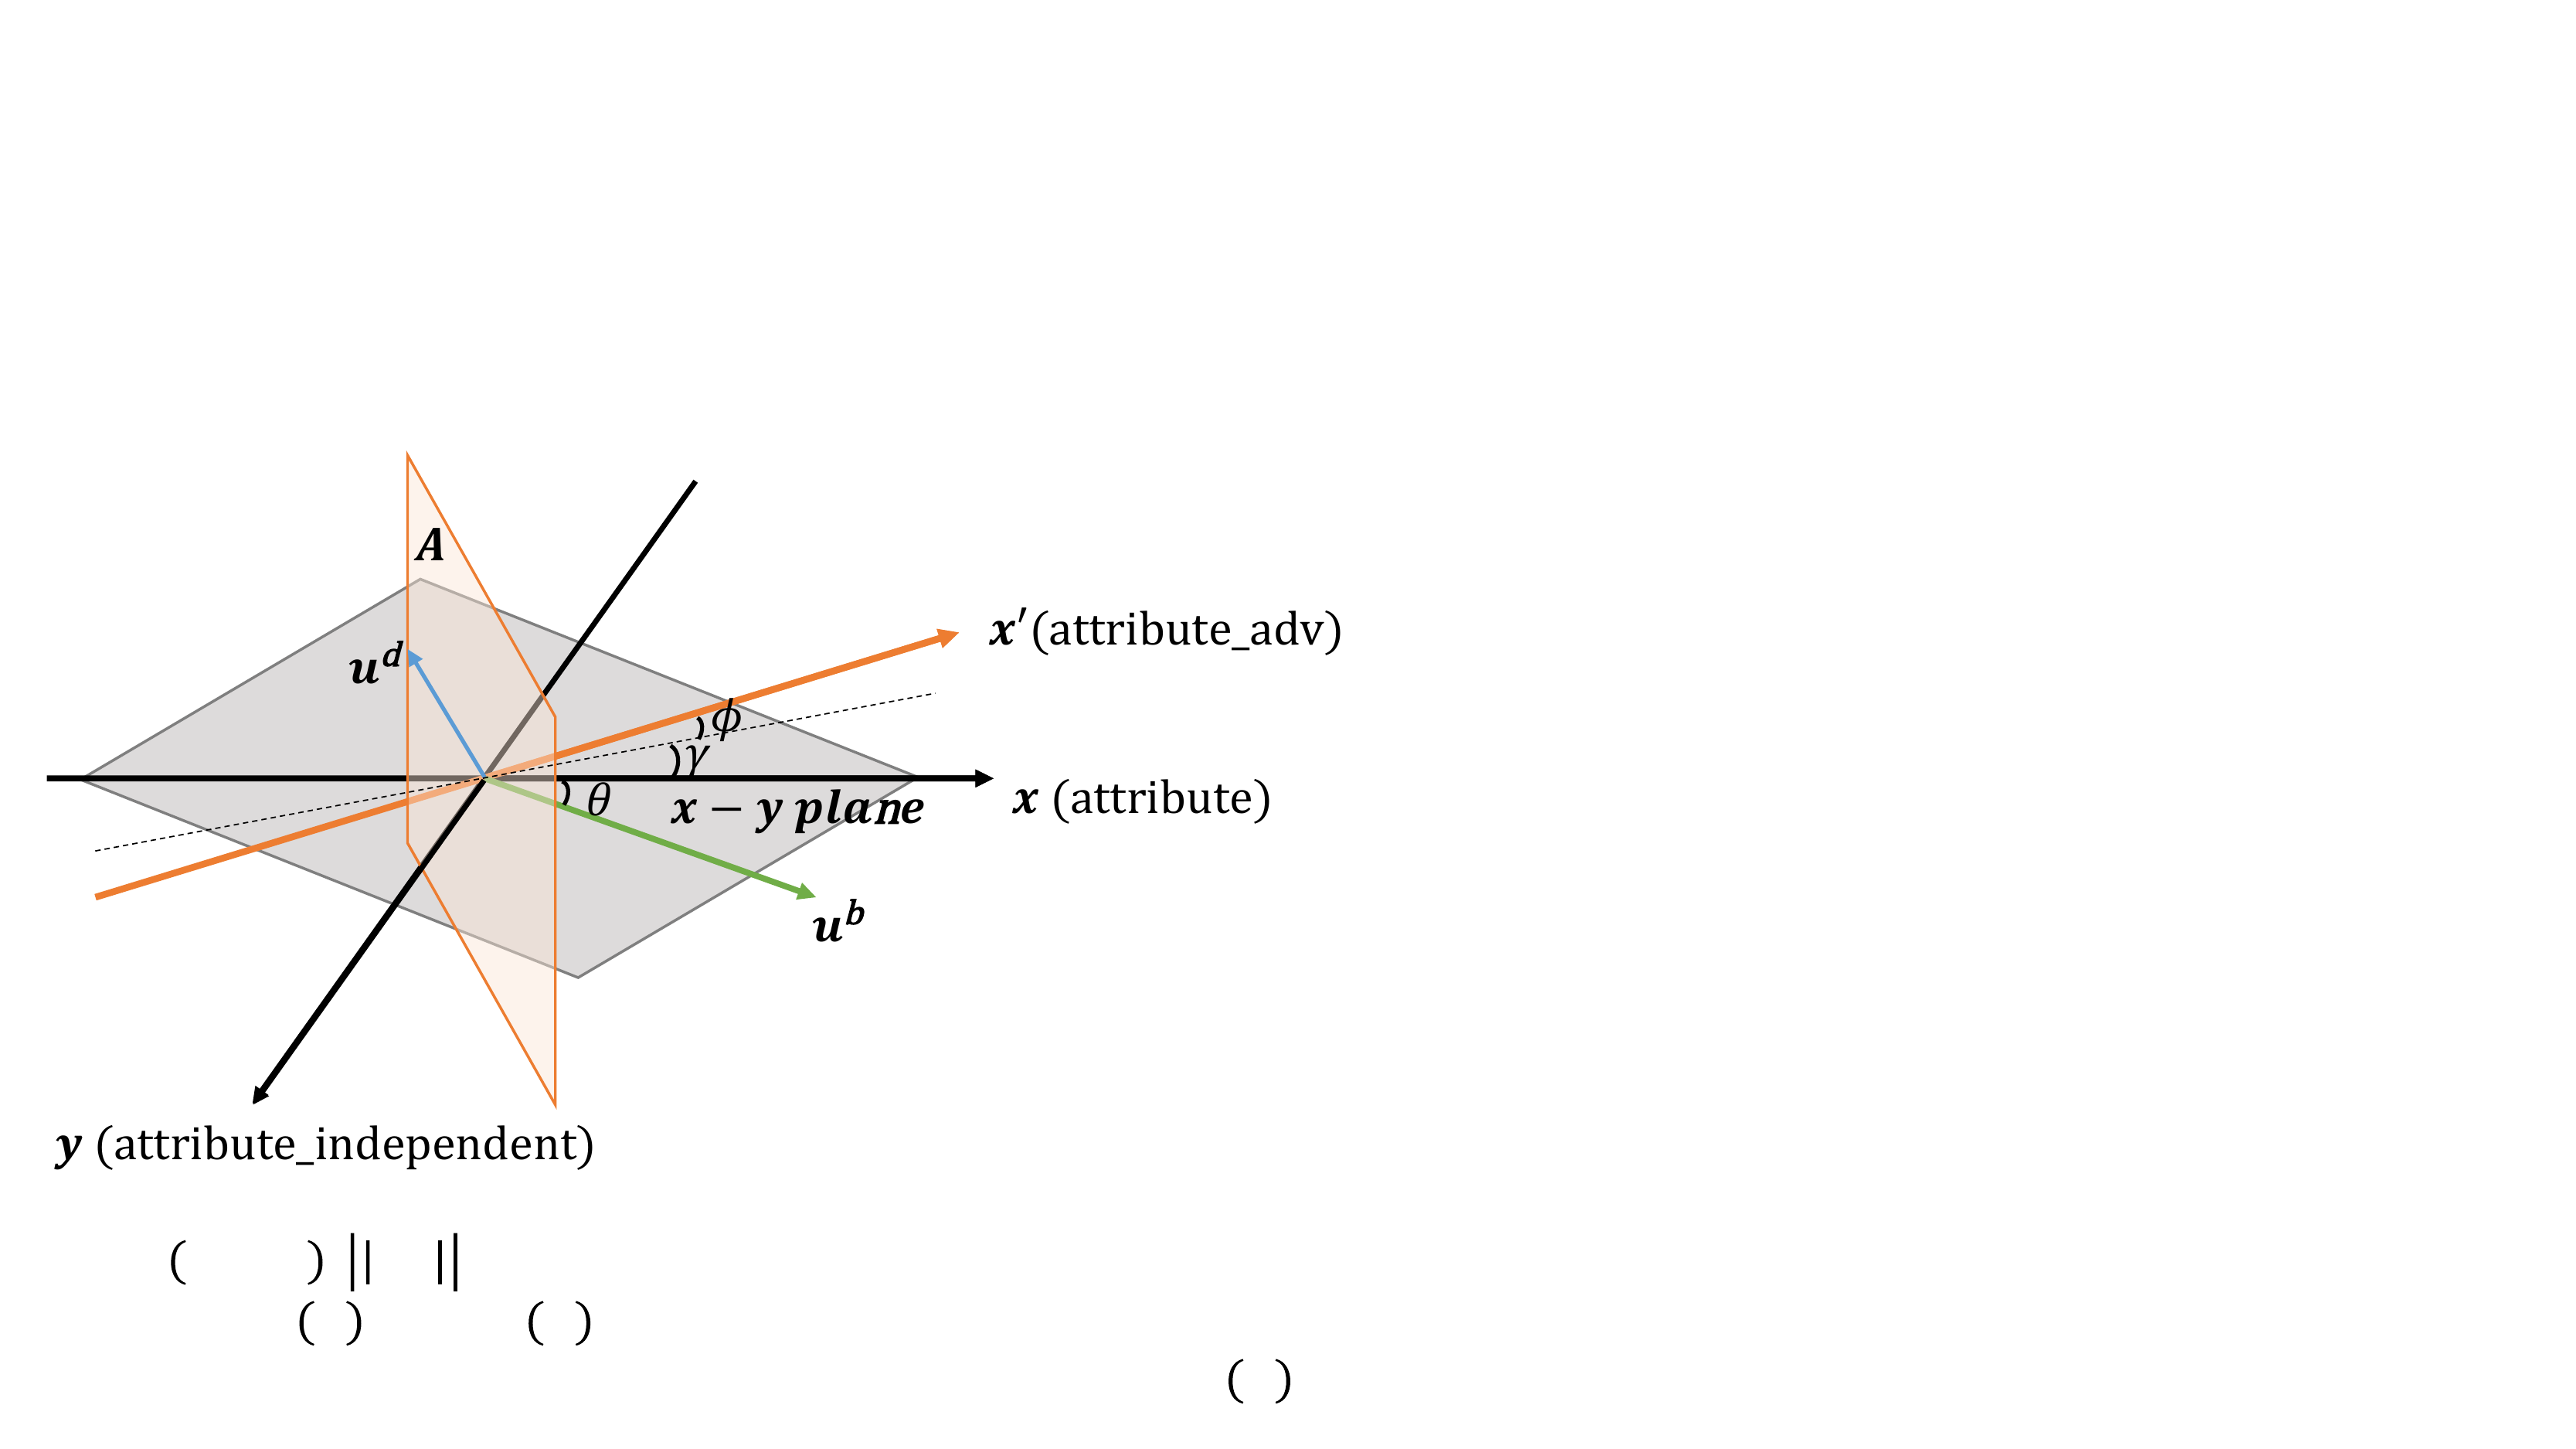}
    }
   %     \subfigure[Orthogonality regularization only.]{\label{analysis2}
 %   \includegraphics[width=0.31\linewidth]{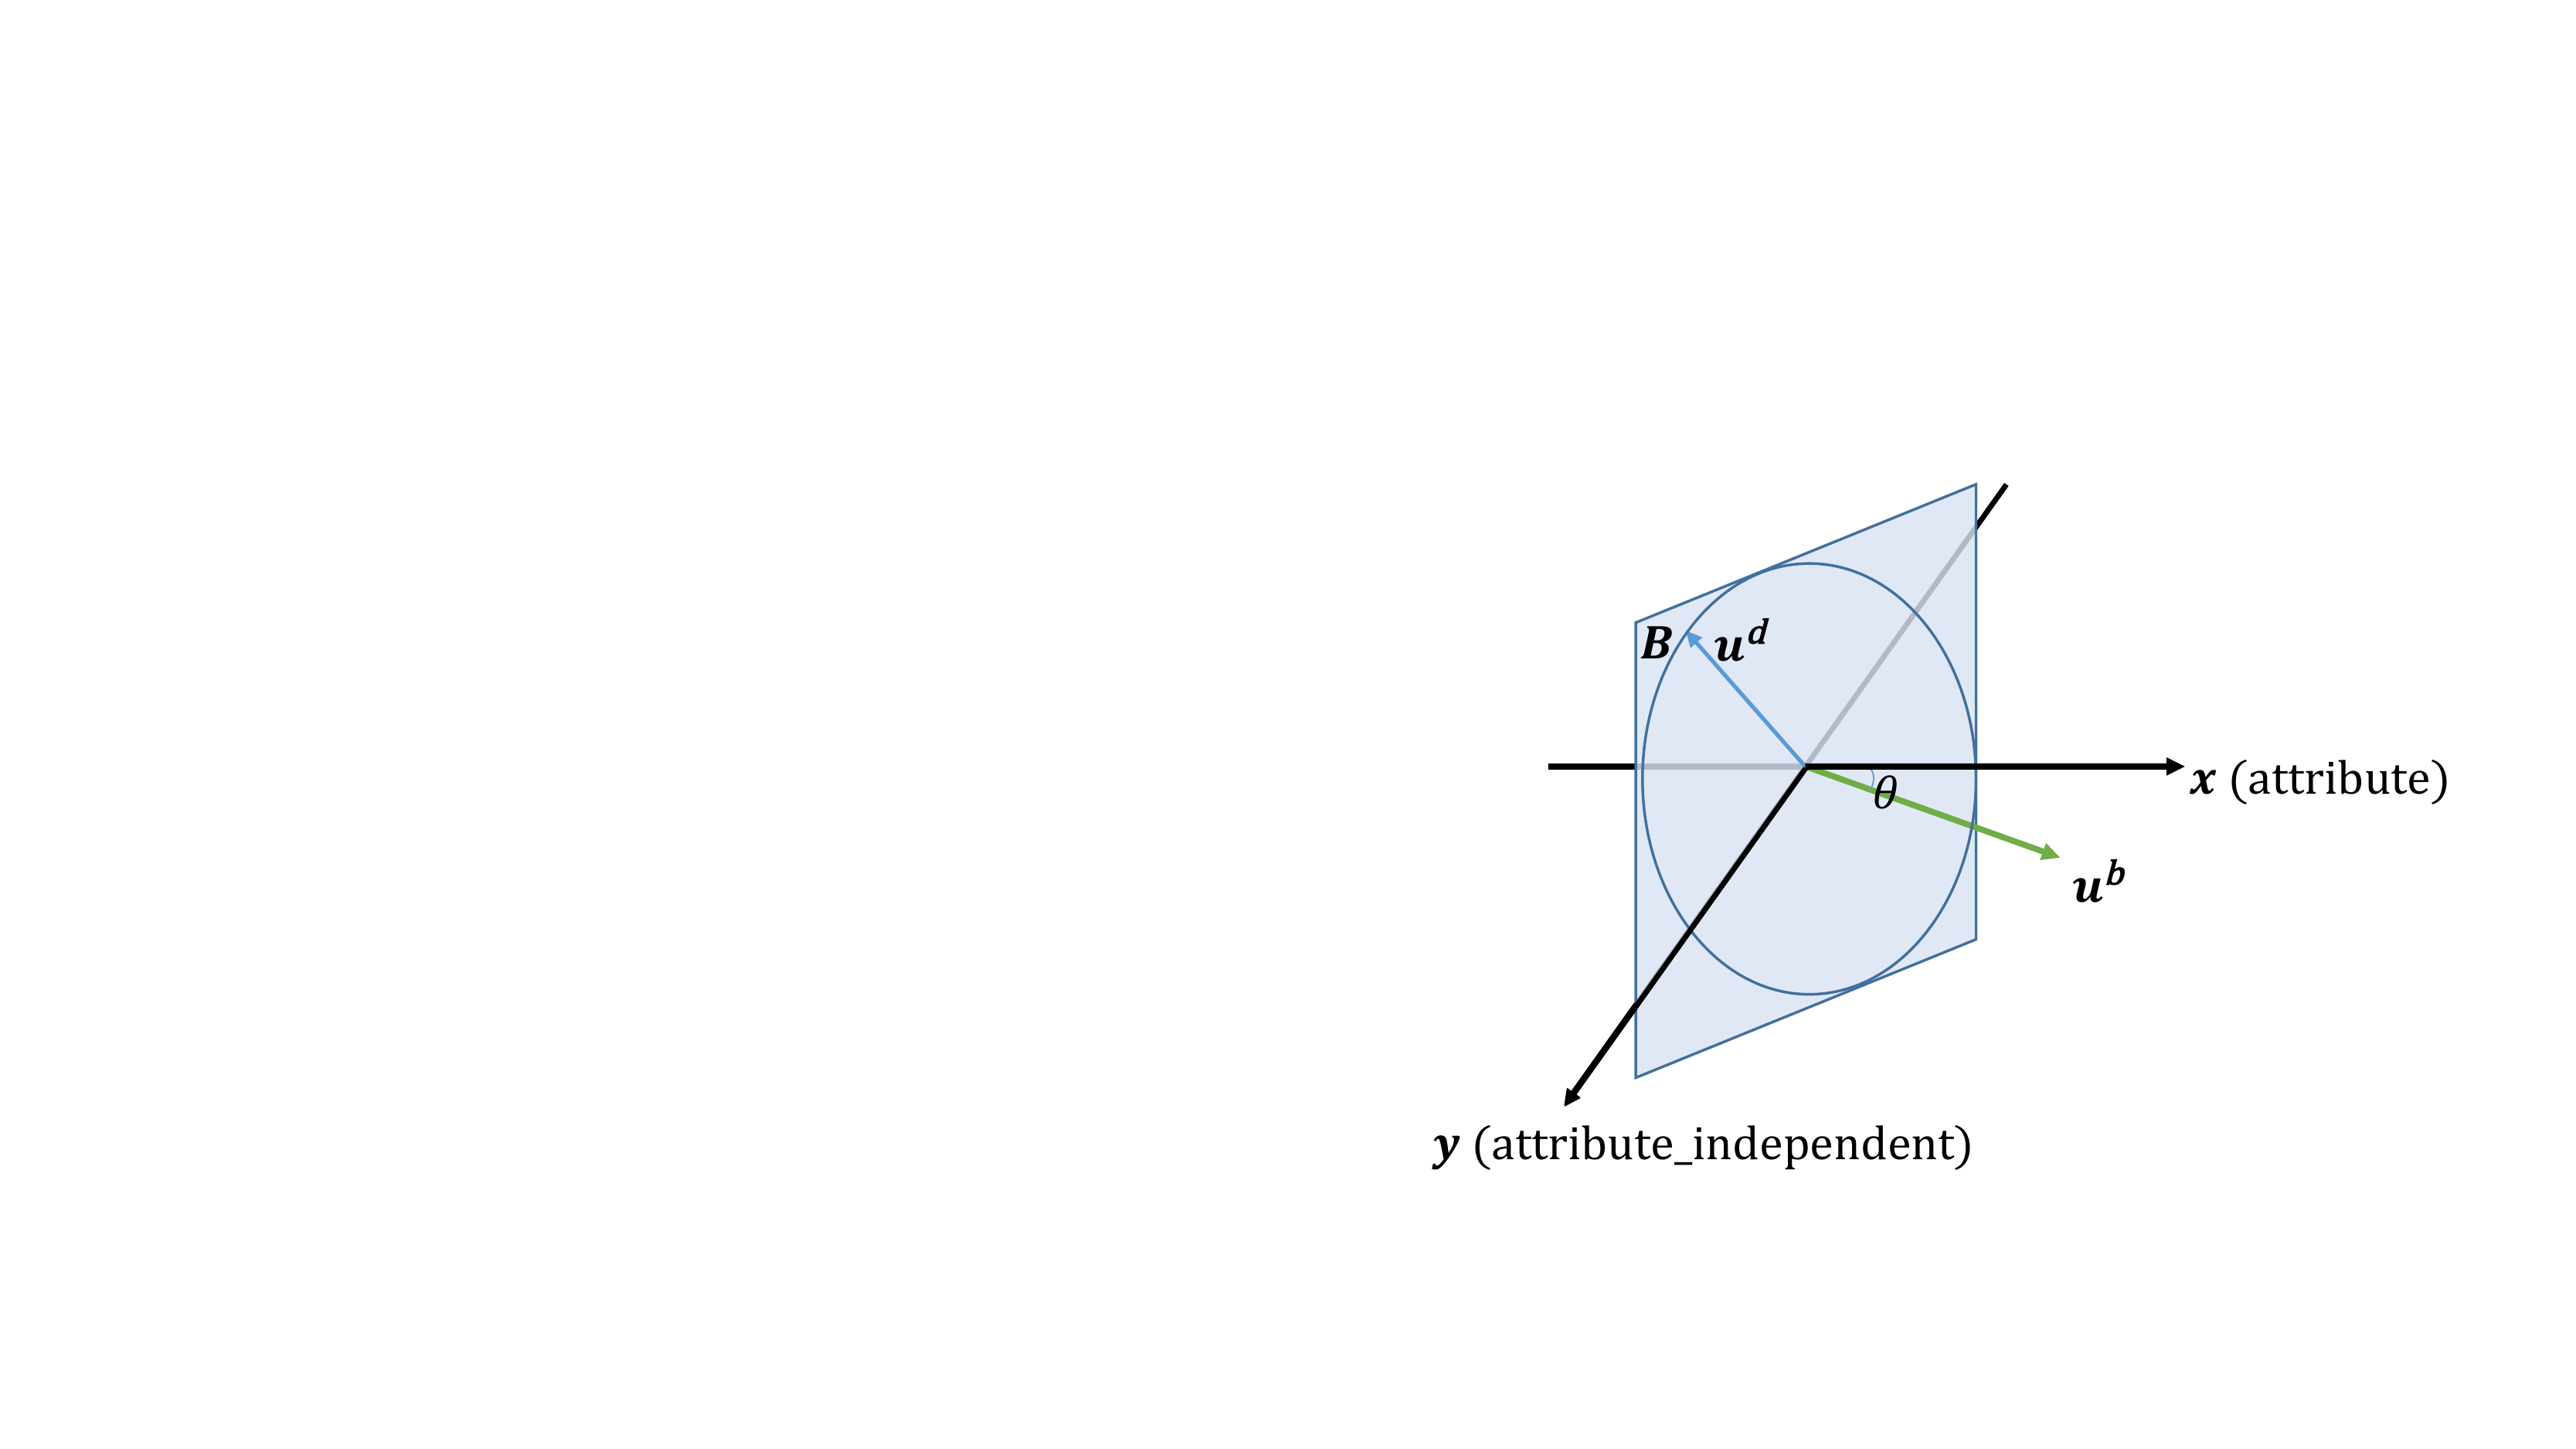}
 %   }
       \subfigure[Our FAN approach.]{\label{analysis3}
    \includegraphics[width=0.98\linewidth]{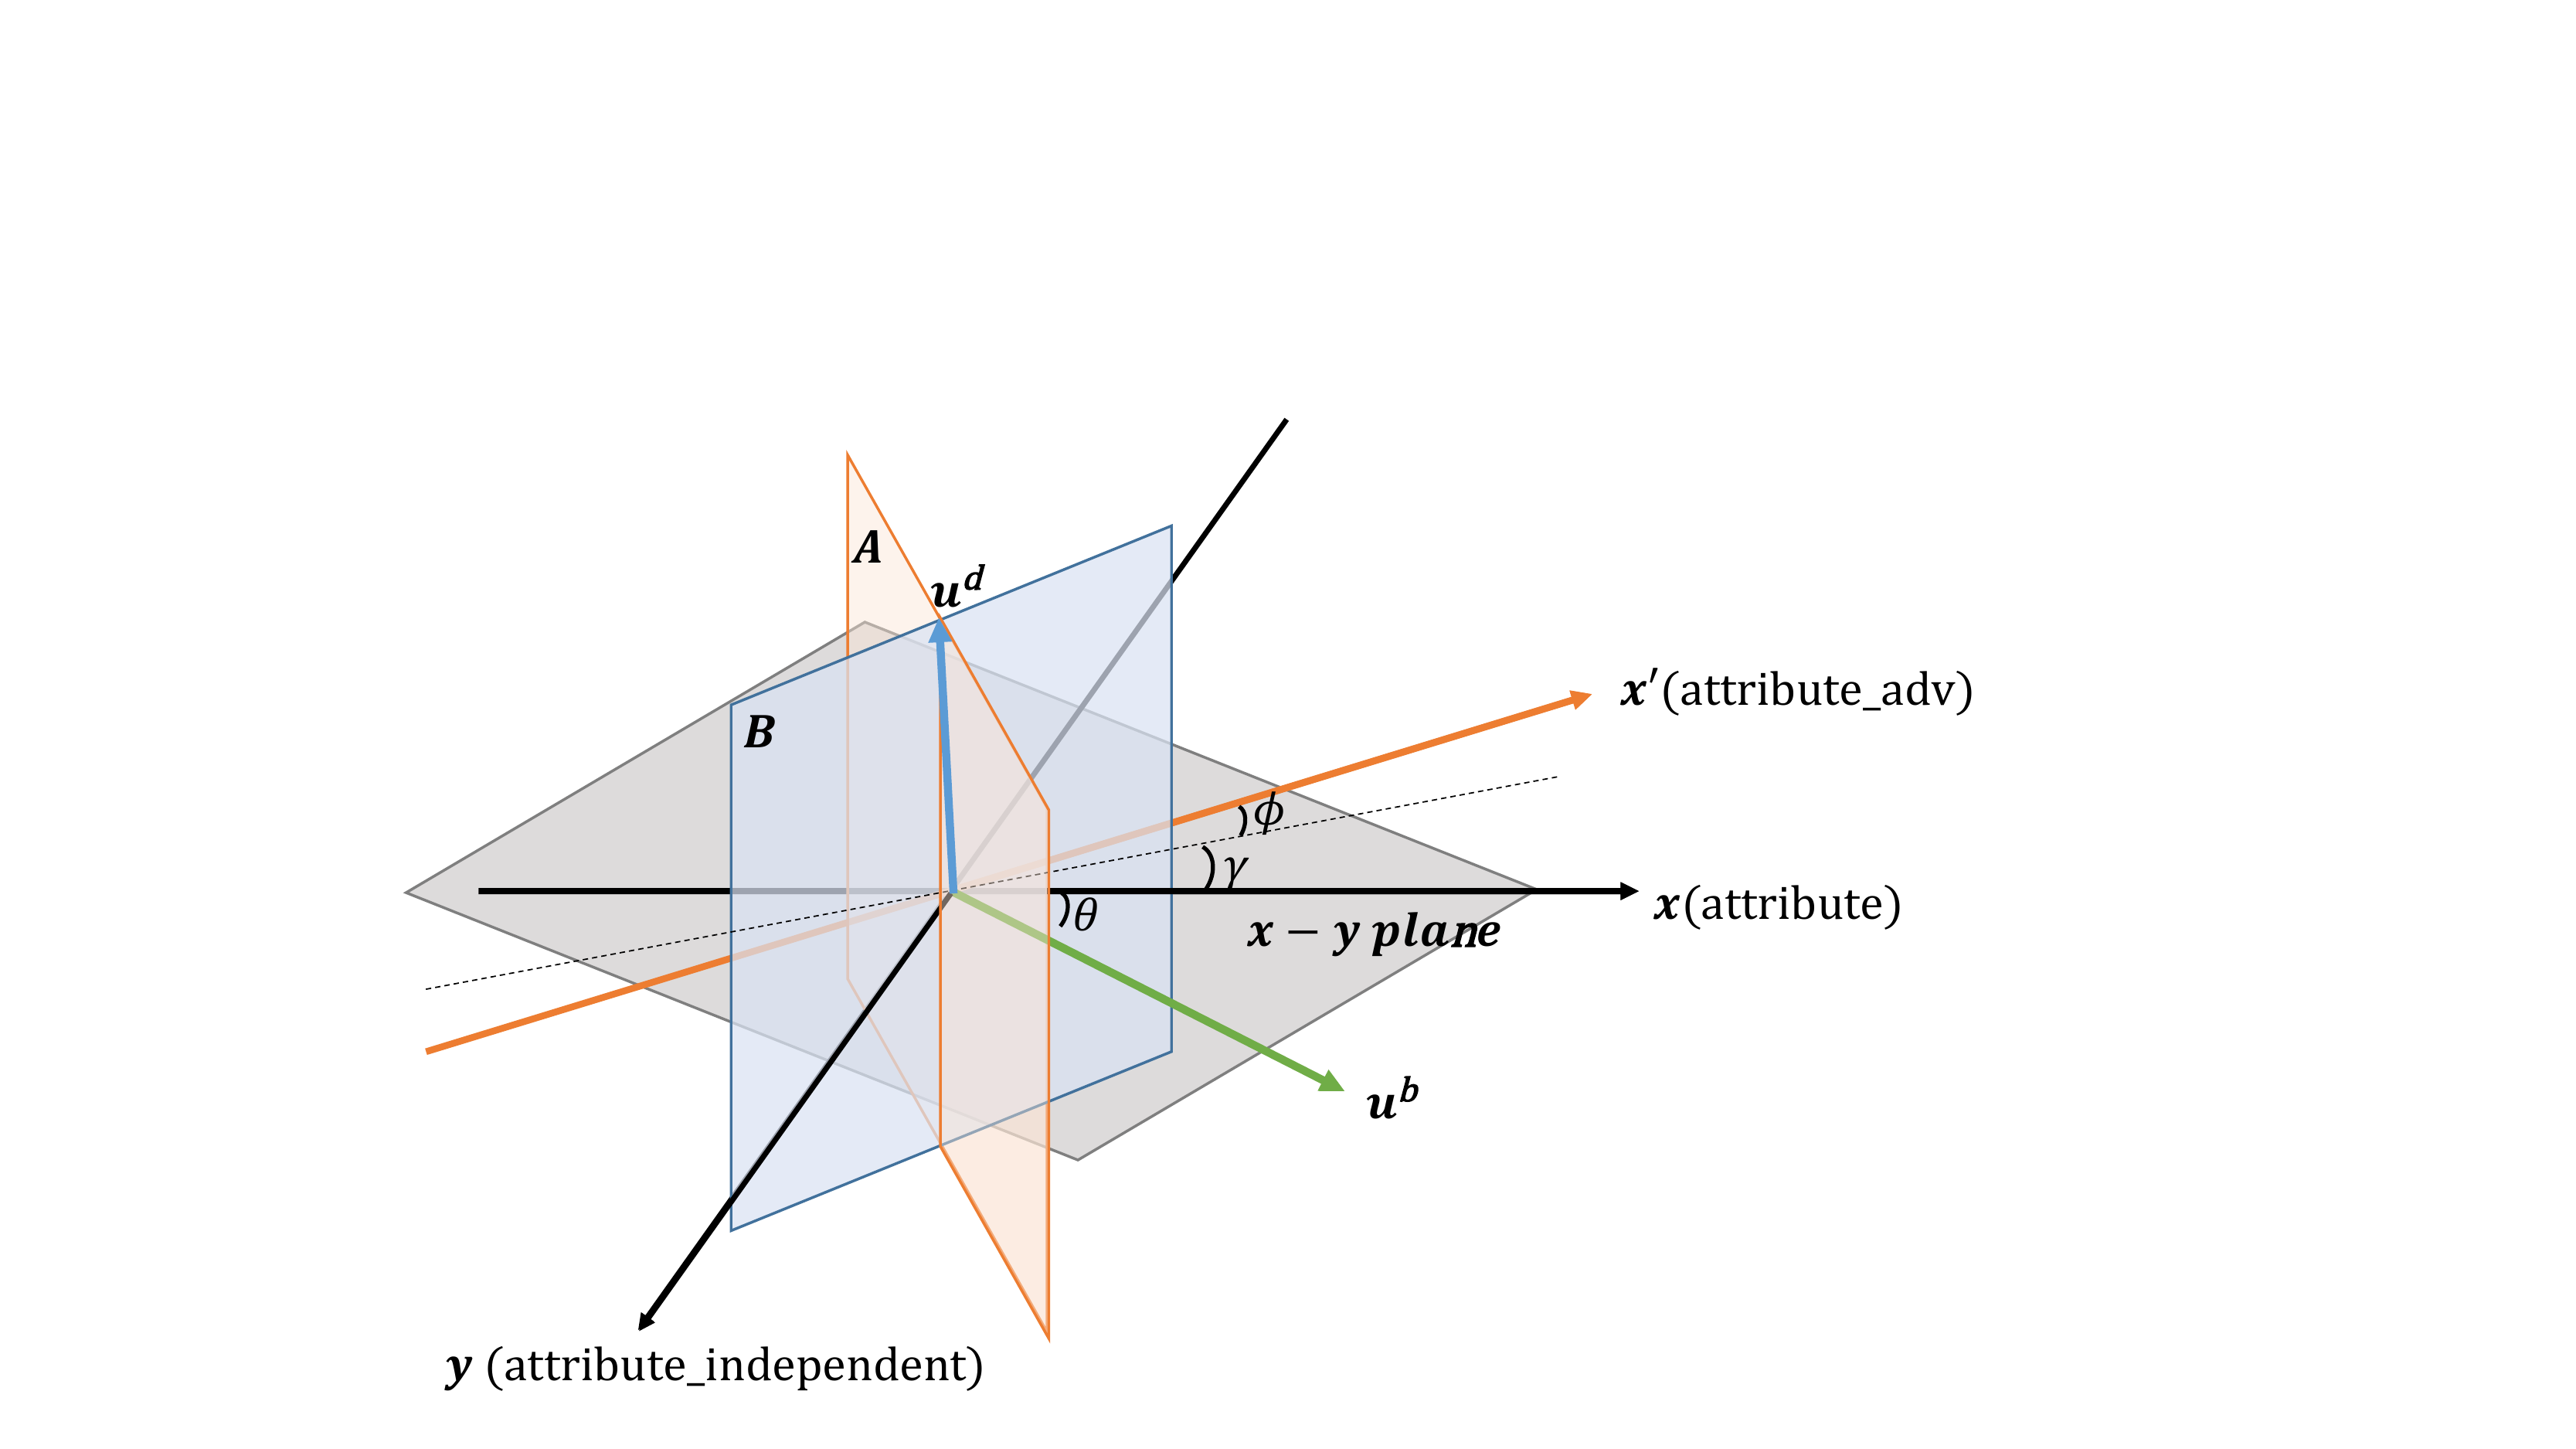}
    }
    \caption{Qualitative analysis of the user embeddings learned by FAN and its variants with adversarial learning only.}
    \label{fig:analysis}
\end{figure}

\begin{table*}[t]
	\centering
\resizebox{0.95\textwidth}{!}{
\begin{tabular}{ccccccccc}
\Xhline{1.5pt}
\multirow{2}{*}{\textbf{Methods}} & \multicolumn{2}{c}{\textbf{Top 1}} & \multicolumn{2}{c}{\textbf{Top 3}} & \multicolumn{2}{c}{\textbf{Top 5}}       & \multicolumn{2}{c}{\textbf{Top 10}} \\ \cline{2-9} 
                                  & Accuracy         & Macro-F         & Accuracy         & Macro-F         & Accuracy       & Macro-F        & Accuracy     & Macro-F     \\ \hline
LibFM           & 62.96$\pm$0.95 & 53.73$\pm$0.89 & 65.13$\pm$0.81 & 60.07$\pm$0.80 & 66.99$\pm$0.76 & 61.69$\pm$0.78 & 68.37$\pm$0.69 & 65.41$\pm$0.66                          \\
%DFM             & 63.74$\pm$0.85 & 54.28$\pm$0.83 & 65.43$\pm$0.80 & 60.38$\pm$0.82 & 67.44$\pm$0.78 & 62.03$\pm$0.79& 68.69$\pm$0.67 & 65.73$\pm$0.66   \\            
EBNR             &63.64$\pm$0.83 & 54.21$\pm$0.82 & 65.51$\pm$0.76 & 60.46$\pm$0.77 & 67.49$\pm$0.75 & 62.06$\pm$0.74& 68.73$\pm$0.69 & 65.75$\pm$0.68                      \\ 
DKN            & 63.66$\pm$0.78 & 54.30$\pm$0.80 & 65.58$\pm$0.79 & 60.52$\pm$0.80 & 67.53$\pm$0.73 & 62.17$\pm$0.73& 68.99$\pm$0.71 & 65.80$\pm$0.72                        \\
DAN            & 63.71$\pm$0.81 & 54.26$\pm$0.79 & 65.59$\pm$0.75 & 60.54$\pm$0.74 & 67.51$\pm$0.74 & 62.19$\pm$0.75& 69.01$\pm$0.70 & 65.83$\pm$0.72                         \\
NPA         & 63.88$\pm$0.82 & 54.34$\pm$0.84 & 65.72$\pm$0.77 & 60.75$\pm$0.75 & 67.59$\pm$0.71 & 62.32$\pm$0.73& 69.14$\pm$0.65 & 65.89$\pm$0.62                       \\
NRMS            & 63.89$\pm$0.86 & 54.40$\pm$0.83 & 65.78$\pm$0.75 & 60.79$\pm$0.76 & 67.64$\pm$0.72 & 62.35$\pm$0.70 & 69.19$\pm$0.63 & 66.01$\pm$0.68        \\ \hline

%FAN-basic     & 63.94$\pm$0.88 & 54.46$\pm$0.85 & 65.97$\pm$0.76 & 60.88$\pm$0.77 & 67.72$\pm$0.70 & 62.43$\pm$0.72 & 69.28$\pm$0.64 & 66.19$\pm$0.65    \\ \hline
MR     & 62.96$\pm$0.91          & 53.48$\pm$0.83        &  64.57$\pm$0.82          & 58.83$\pm$0.81          & 66.19$\pm$0.73                           & 60.82$\pm$0.70     & 68.36$\pm$0.65    & 65.12$\pm$0.67              \\
AL     & 62.55$\pm$0.85          & 52.80$\pm$0.83        &  63.31$\pm$0.74          & 57.62$\pm$0.75          & 65.43$\pm$0.68                           & 59.88$\pm$0.66     & 66.86$\pm$0.62    & 63.55$\pm$0.61                           \\
ALGP     & 62.48$\pm$0.86          & 52.72$\pm$0.82        &  63.09$\pm$0.75          & 57.31$\pm$0.73          & 65.21$\pm$0.66                           & 59.43$\pm$0.67     & 66.16$\pm$0.61    & 63.28$\pm$0.63              \\
\hline

FAN     & \textbf{62.10}$\pm$0.80          & \textbf{52.41}$\pm$0.76        &  \textbf{62.61}$\pm$0.69          & \textbf{54.36}$\pm$0.68          & \textbf{62.95}$\pm$0.62                           & \textbf{55.98}$\pm$0.63     & \textbf{63.39}$\pm$0.59    & \textbf{57.13}$\pm$0.58                           \\ \hline
Random*    & 62.08$\pm$0.91          & 52.39$\pm$0.90   &  62.57$\pm$0.79          & 54.27$\pm$0.79    & 62.86$\pm$0.78          & 55.91$\pm$0.76  & 63.12$\pm$0.68 &  56.97$\pm$0.67                                  \\
\Xhline{1.5pt}
\end{tabular}
}
	\caption{News recommendation fairness of different methods on real impression logs. Lower scores indicate better fairness. The best results except random ranking are in bold. *Randomly ranked impressions are still gender discriminative because the impression logs contain system gender bias introduced by the personalized recall and ranking process.}\label{table.result3}
\end{table*}

\subsection*{Discussions on Decomposed Adversarial Learning}\label{sec.discussion}

In this section, we present several qualitative discussions on the intuition and effectiveness of our decomposed adversarial learning method  with orthogonality regularization.
We consider a simplified case to discuss the characteristics of user embeddings learned by our FAN approach and its variants with adversarial learning only, as shown in Fig.~\ref{fig:analysis}.
In this case, we assume that user attribute is a binary variable and the probability score can be obtained by $\hat{z}=sigmoid(\mathbf{x}\cdot \mathbf{u})$, which means that the attribute is easier to be inferred from $\mathbf{u}$ when the projection of $\mathbf{u}$ on the x-axis is longer, while cannot be discriminated when $\mathbf{u}$ is orthogonal to the x-axis.
Since the user attribute usually cannot be perfectly inferred from user embeddings, we assume that the bias-aware user embedding $\mathbf{u}^b$ is spanned by the attribute space $x$ and an attribute-independent space $y$ (shown as the y-axis), which is denoted as $\mathbf{u}^b=C[\cos(\theta)\mathbf{x}+\sin(\theta)\mathbf{y}]$, where $\theta$ is the angle between $\mathbf{u}^b$ and the x-axis and $C$ is the norm of $\mathbf{u}^b$.  

The case with only adversarial learning applied to the bias-free user embedding is illustrated in Fig.~\ref{analysis1}. 
Since the decision boundary of the discriminator (illustrated as the x'-axis) may have shifts with the real attribute space (x-axis), we denote the angle of the projections of two axes on the x-y plane as $\gamma$.
In addition, the x'-axis may even have some shifts with the x-y plane, and we denote their angle as $\phi$.
We can see that if the adversarial learning reaches a Nash equilibrium, the bias-free user embedding $\mathbf{u}^d$ should be orthogonal to the x'-axis and is limited on the plane $A$.
Considering an ideal case when $\phi=0$, then the projection length of $\mathbf{u}^d$ on the x-axis can be only bounded by:
\begin{equation}
    |\mathbf{x}\cdot \mathbf{u}^d|\leq ||\mathbf{u}^d||\sin(\gamma),  \label{eq2}
\end{equation}
where $||\mathbf{u}^d||$ can be regarded as a constant.
This formula shows that unbiased user representations can only be learned when the attribute is very easy to be predicted, and there is no guarantee that the bias can be effectively eliminated when the user embeddings are not attribute discriminative.
%In addition, if $\phi$ is very large (e.g., $\phi=\pi/2$), the method will fail.
Thus, we cannot use adversarial learning only to achieve fair news recommendation, since user attributes usually cannot be perfectly recovered from news click behaviors~\cite{wu2019neural}.

%Then, we consider the model with orthogonality regularization only, which is analyzed in Fig.~\ref{analysis2}.
%Due to the orthogonality regularization, the bias-free user embedding can be almost orthogonal to the bias-aware user embedding.\footnote{This loss is less than 1e-2 in our experiments, indicating that both user embeddings are nearly orthogonal.}
%Thus, the bias-free user embedding is approximately on a plane $B$ that is orthogonal to the biased user embedding $\mathbf{u}^b$.
%In this case, the projection length of $\mathbf{u}^d$ on the x-axis is only bounded by:
%\begin{equation}
%    |\mathbf{x}\cdot \mathbf{u}^d|\leq ||\mathbf{u}^d||\sin(\theta). \label{eq3}
%\end{equation}
%This boundary also indicates that the user attribute information may not be sufficiently removed from the bias-free user embedding when the user attribute is difficult to be inferred.  
%Thus, we also cannot only use the orthogonality regularization to achieve fair news recommendation.

Then, we discuss our FAN approach with orthogonality regularization in Fig.~\ref{analysis3}.
Due to the orthogonality regularization, the bias-free user embedding can be almost orthogonal to the bias-aware user embedding.\footnote{This loss is less than 1e-2 in our experiments, indicating that both user embeddings are nearly orthogonal.}
Thus, the bias-free user embedding is approximately on a plane $B$ that is orthogonal to the bias-aware user embedding $\mathbf{u}^b$.
When the adversarial learning achieves a Nash equilibrium, the bias-free user embedding is approximately the intersection of the planes $A$ and $B$, i.e., $\mathbf{u}^d \approx A\cap B$.
Then, the projection length of $\mathbf{u}^d$ on the x-axis is bounded by:
\begin{equation}
    |\mathbf{x}\cdot \mathbf{u}^d|\leq ||\mathbf{u}^d||\sin(\theta)\sin(\phi), \label{eq4}
\end{equation}
which is much smaller than the boundaries in Eq. (\ref{eq2}), and is independent on the shift $\gamma$ of the discriminator on the x-y plane.
Thus, the bias information in the bias-free user embedding can be better removed, which means that our approach can achieve better recommendation fairness than using adversarial learning only.
